# Supplementary material for: Recovery of dynamic interference
Source: arXiv:1611.04116 ancillary file (2016-11-13)
Supplement: Supplementary file 1 [file recovery-suppl.pdf]

# Supplement for "Recovery of dynamic interference"

Mehrdad Baghery, Ulf Saalmann & Jan M. Rost

A detailed derivation of some (largely known) basic analytical expressions is provided. Firstly, we give explicit expressions for the two dimensionless parameters $\delta$ and $\gamma$ describing respectively the dynamic Stark shift and the depletion of some state in a high-frequency laser pulse, followed by their asymptotic behaviour. Secondly, we show how the Stark shifts in different gauges are related. Thirdly, we outline the numerical procedure for propagation of the TDSE, and stress convergence problems in the length gauge by comparing the results of a few systematic simulations (with an increasing number of partial waves included in the propagation) in the velocity and length gauges.

## 1 Stark shift and depletion in single-photon ionization

In order to explain the notation used in the text[1], in this section we will describe the Stark shift and the depletion of an initial state upon irradiation with a high-frequency laser pulse. The ideas presented here largely follow those presented before [1], followed by further definitions and a general discussion.

The wavefunction evolving according to the time-dependent Schrödinger equation

$$\mathrm{i}\frac{\partial}{\partial t}\big|\psi(t)\big\rangle = \hat{H}(t)\big|\psi(t)\big\rangle \quad \text{with} \quad \hat{H}(t) = \frac{1}{2}\big[\hat{\mathbf{p}} + \boldsymbol{\mathcal{A}}(t)\big]^2 + V(\hat{\mathbf{r}}) \quad \text{and} \quad \boldsymbol{\mathcal{A}}(t) = \boldsymbol{\mathcal{A}}_0\, g(t)\cos(\omega t) \tag{S1}$$

can be expanded in terms of field-free states, cf. ansatz (2) in the text. The amplitude of the initially occupied state $\varphi_{\mathrm{in}}$, and all the bound/continuum states $\varphi_\alpha$ having a non-vanishing coupling $\mathbf{p}_\alpha = \langle\varphi_\alpha|\hat{\mathbf{p}}|\varphi_{\mathrm{in}}\rangle$ with the initial state respectively reads

$$\mathrm{i}\frac{\mathrm{d}}{\mathrm{d}t}a_{\mathrm{in}}(t) = g(t)\sum\!\!\!\!\!\!\int_\alpha \boldsymbol{\mathcal{A}}_0\cdot\frac{\mathbf{p}_\alpha^{\,*}}{2}\sum_\pm \mathrm{e}^{\mathrm{i}[E_{\mathrm{in}}\pm\omega-E_\alpha]t}a_\alpha(t), \tag{S2a}$$

$$\mathrm{i}\frac{\mathrm{d}}{\mathrm{d}t}a_\alpha(t) = g(t)\,\boldsymbol{\mathcal{A}}_0\cdot\frac{\mathbf{p}_\alpha}{2}\sum_\pm \mathrm{e}^{\mathrm{i}[E_\alpha\pm\omega-E_{\mathrm{in}}]t}a_{\mathrm{in}}(t). \tag{S2b}$$

Assuming that the envelope changes slowly, i. e. $\frac{\mathrm{d}}{\mathrm{d}t}g(t)\approx 0$, which implies $\frac{\mathrm{d}}{\mathrm{d}t}a_{\mathrm{in}}(t)\approx 0$, one can solve Eq. (S2b) approximately to get

$$a_\alpha(t) \approx -g(t)\,\boldsymbol{\mathcal{A}}_0\cdot\frac{\mathbf{p}_\alpha}{2}\sum_\pm\frac{\mathrm{e}^{\mathrm{i}[E_\alpha-E_{\mathrm{in}}\pm\omega]t}}{E_\alpha-E_{\mathrm{in}}\pm\omega}a_{\mathrm{in}}(t). \tag{S3}$$

This can be in turn used in Eq. (S2a) to get the following equation for the initial amplitude

$$\frac{\mathrm{d}}{\mathrm{d}t}a_{\mathrm{in}}(t) = -\mathrm{i}E_{\mathrm{p}}(t)\big[\delta-\mathrm{i}\gamma/2\big]a_{\mathrm{in}}(t) \qquad \text{with} \quad E_{\mathrm{p}}(t)\equiv\frac{\mathcal{A}_0^2}{4}g^2(t), \tag{S4a}$$

[1]Here and in the following we use "text" when referring to the text of main manuscript.

where terms with $e^{\pm i2\omega t}$ have been neglected and the following definitions have been used

$$\delta \equiv -\sum\!\!\!\!\!\!\int_\alpha \sum_\pm \frac{\widetilde{p}_\alpha^{\,2}}{E_\alpha - E_{\rm in} \pm \omega} = \sum\!\!\!\!\!\!\int_\alpha \widetilde{p}_\alpha^{\,2} \frac{2[E_\alpha - E_{\rm in}]}{\omega^2 - [E_\alpha - E_{\rm in}]^2} \tag{S4b}$$

$$\gamma \equiv 2\pi \int \mathrm{d}E_\alpha \, \delta\big(E_\alpha - [E_{\rm in} + \omega]\big)\, \widetilde{p}_\alpha^{\,2} = 2\pi\, \widetilde{p}_\omega^{\,2} \quad \text{with } E_\omega = E_{\rm in} + \omega \tag{S4c}$$

$$\widetilde{p}_\alpha \equiv \frac{\boldsymbol{\mathcal{A}}_0}{|\boldsymbol{\mathcal{A}}_0|} \cdot \mathbf{p}_\alpha, \tag{S4d}$$

with the integral part of Eq. (S4b) being understood as Cauchy principal value.

Such equations have been derived before [1], but here $\delta$ and $\gamma$ are defined slightly differently such that they are solely determined by the system (and the frequency). In particular, we have taken out the instantaneous ponderomotive energy $E_{\rm p}(t)$ which depends on time through the pulse envelope $g(t)$ as defined in Eq. (S4a).

### 1.1 Asymptotic behavior and condition for dynamic interference

The asymptotic behavior of $\delta$ and $\gamma$ at large frequencies $\omega$ is given by

$$\delta \approx 2 \sum_\alpha \frac{[E_\alpha - E_{\rm in}]\, \widetilde{p}_\alpha^{\,2}}{\omega^2} \sim \omega^{-2} \tag{S5a}$$

$$\gamma \sim \sqrt{\omega}\left[\omega \frac{8\sqrt{2\omega}}{[1+2\omega]^3}\right]^2 \sim \omega^{-5/2}. \tag{S5b}$$

where in the first step of Eq. (S5a) we have restricted the sum to bound states since their coupling matrix elements are much larger than those of the continuum states. In the second step we have assumed $E_\alpha - E_{\rm in} \ll \omega$.

In order to get Eq. (S5b), we note that at high frequencies $\omega$ (and thus high energies $E_\alpha$) the electron can be considered free and therefore its radial wavefunction becomes $\varphi_\alpha \sim [2E_\alpha]^{1/4} j_1(\sqrt{2E_\alpha} r) \approx [2\omega]^{1/4} j_1(\sqrt{2\omega} r)$, with $j_1$ being the 1st-order spherical Bessel function. This allows for an easy analytical integration with the result shown above.

As becomes clear from these considerations, one always ends up with $\gamma < \delta$ in the limit of $\omega \to \infty$ regardless of the system. In other words, for any system there is always a crossover frequency $\widetilde{\omega}$, however large, above which $\gamma(\omega) < \delta(\omega)$. Thus — in principle — dynamic interference can be observed for appropriate laser parameters.

Considering a hydrogen-like atom with nuclear charge $Z$, one gets related quantities

$$\delta_Z(\omega) = Z^{-4}\, \delta(Z^2\omega), \quad \gamma_Z(\omega) = Z^{-4}\, \gamma(Z^2\omega) \tag{S6}$$

by simple scaling arguments. Visibly the transition to $\delta_Z(\omega) > \sqrt{\pi}\, \gamma_Z(\omega)$ occurs for $Z > 1$ at a $Z^2$–times larger frequency and is connected with a $Z^4$–times larger product $E_{\rm p}\, T$, cf. Eqs. (5) and (6) in the text.

## 2 Dynamic Stark shift

We summarize formulas for the dynamic Stark shift (often referred to as AC Stark shift) and discuss the Stark of the ground and an excited state of the hydrogen atom.

### 2.1 Length vs. velocity gauge

Given the three Hamiltonians [2]

$$\hat{H}^{\rm red} = \frac{1}{2}\hat{\mathbf{p}}^2 + \boldsymbol{\mathcal{A}}(t)\hat{\mathbf{p}} + V(\hat{\mathbf{r}}) \tag{S7a}$$

$$\hat{H}^{\rm vel} = \frac{1}{2}\big[\hat{\mathbf{p}} + \boldsymbol{\mathcal{A}}(t)\big]^2 + V(\hat{\mathbf{r}}) \tag{S7b}$$

$$\hat{H}^{\rm len} = \frac{1}{2}\hat{\mathbf{p}}^2 + V(\hat{\mathbf{r}}) - \frac{\mathrm{d}}{\mathrm{d}t}\boldsymbol{\mathcal{A}}(t)\cdot\hat{\mathbf{r}} \tag{S7c}$$

and the initial conditions $\big|\psi^{\rm len}(-\infty)\big\rangle = \big|\psi^{\rm vel}(-\infty)\big\rangle = \big|\psi^{\rm red}(-\infty)\big\rangle$, the solutions of the time-dependent Schrödinger equation for $\xi = \mathrm{len}, \mathrm{vel}, \mathrm{red}$

$$\mathrm{i}\frac{\partial}{\partial t}\big|\psi^{\xi}(t)\big\rangle = \hat{H}^{\xi}\big|\psi^{\xi}(t)\big\rangle \tag{S8}$$

are connected by

$$\big|\psi^{\rm vel}(t)\big\rangle = \mathrm{e}^{-\frac{\mathrm{i}}{2}\int^t \mathrm{d}t' \boldsymbol{\mathcal{A}}^2(t')}\big|\psi^{\rm red}(t)\big\rangle, \tag{S9a}$$

$$\big|\psi^{\rm len}(t)\big\rangle = \mathrm{e}^{+\mathrm{i}\boldsymbol{\mathcal{A}}(t)\cdot\hat{\mathbf{r}}}\big|\psi^{\rm vel}(t)\big\rangle. \tag{S9b}$$

Note that $\big|\psi^{\rm len}(t_*)\big\rangle = \big|\psi^{\rm vel}(t_*)\big\rangle$ every time when $\mathcal{A}(t_*) = 0$, i.e. both states agree periodically. $\big|\psi^{\rm vel}(t)\big\rangle$ and $\big|\psi^{\rm red}(t)\big\rangle$ differ only by a trivial phase $\mathrm{e}^{-\frac{\mathrm{i}}{2}\int^t \mathrm{d}t' \mathcal{A}^2(t')}$ introduced in Eq. (2) of the text.

By means of the 2nd-order perturbation theory one can calculate the Stark shift of an eigenstate $\varphi_*$ in terms of all (bound and continuum) eigenstates in the three cases as follows [2], cf. also Eq. (S4b) above,

$$\Delta^{\rm red}(t) = E_{\rm p}(t) \sum\!\!\!\!\!\!\!\int_{\alpha} \big|\big\langle\varphi_\alpha\big|\hat{\mathbf{p}}\big|\varphi_*\big\rangle\big|^2 \frac{2E_{\alpha *}}{\omega^2 - E_{\alpha *}{}^2}, \tag{S10a}$$

$$\Delta^{\rm vel}(t) = \Delta^{\rm red}(t) + E_{\rm p}(t), \tag{S10b}$$

$$\Delta^{\rm len}(t) = E_{\rm p}(t) \sum\!\!\!\!\!\!\!\int_{\alpha} \big|\big\langle\varphi_\alpha\big|\hat{\mathbf{r}}\big|\varphi_*\big\rangle\big|^2 \frac{2E_{\alpha *}}{1 - E_{\alpha *}{}^2/\omega^2}. \tag{S10c}$$

where the abbreviation $E_{\alpha *} \equiv E_\alpha - E_*$ is used. As above, $E_{\rm p}(t)$ is the instantaneous ponderomotive energy which changes in time because of the pulse envelope $g(t)$.

By means of the identity $\langle\varphi_\alpha|\hat{\mathbf{p}}|\varphi_*\rangle = \mathrm{i}E_{\alpha *}\langle\varphi_\alpha|\hat{\mathbf{r}}|\varphi_*\rangle$ for the matrix elements and the TRK sum rule [3], $1 = 2\sum_\alpha E_{*\alpha}|\langle\varphi_\alpha|\hat{\mathbf{r}}|\varphi_*\rangle|^2$, it is easy to show that $\Delta^{\rm vel} = \Delta^{\rm len}$. It turns out, the Stark shift in the length gauge always contains (in a non-separable way) the ponderomotive shift $E_{\rm p}(t)$, whereas in the velocity gauge the ponderomotive shift can be easily taken out simply by neglecting $\frac{1}{2}\mathcal{A}^2(t)$ in the Hamiltonian (S7b) and using (S7a) instead. All three expressions (S10) are shown schematically in Fig. 1 of the text.

The Stark shifts in the various gauges are written in (S10) in a form that suggests

$$\Delta^{\xi}(t) = \delta^{\xi}\, E_{\rm p}(t), \tag{S11}$$

where again $\xi = \mathrm{len}, \mathrm{vel}, \mathrm{red}$, and $\delta^{\xi}$ are the dimensionless parameters introduced in Sec. 1 above and used throughout the text.

### 2.2 Hydrogen atom

The dynamic Stark shift of the hydrogen ground-state is typically positive at large frequencies $\omega > |E_*|$ with $E_*$ being the ground-state energy. This can be easily seen in Eqs. (S10) where the dominating states (those with $E_\alpha \approx E_*$ which also happen to have the largest dipole matrix elements) have a positive denominator as well as a positive numerator, whereas contributions from states with a negative denominator ($E_\alpha \gtrsim E_* + \omega$) are suppressed in two ways: firstly these states have small dipole matrix elements, and secondly they are largely canceled out by those with $E_\alpha \lesssim E_* + \omega$. Therefore the sketch shown in Fig. 1 of the text does not just apply to hydrogen in the 1s-state but is typically for any ground-state atom.

The 2p-state has a negative term in the sum from the coupling to the 1s-state for frequencies $\omega > E_{2p} - E_{1s}$ (negative numerator and positive denominator). Depending on how close $\omega$ is to the 1s-2p transition energy, the total sum (and thus the observed dynamic Stark shift) can be negative or positive. This allows one, by choosing $\omega = 12\,\text{eV}$, to have $\delta^{\text{len}} = \delta^{\text{vel}} = 0$ and consequently $\Delta^{\text{len}}(t) = \Delta^{\text{vel}}(t) = 0$. Hence, the effective Stark shift is $\delta^{\text{red}} = -1$, and therefore $\Delta^{\text{red}}(t) = -E_{\text{p}}(t)$, cf. (S10b). This means that in this case the (negative) Stark shift *increases* the transition energy from the 2p to any continuum state by the instantaneous ponderomotive energy $E_{\text{p}}(t)$. This explains the red-shift observed while increasing the intensity as seen in Fig. 3 of the text.

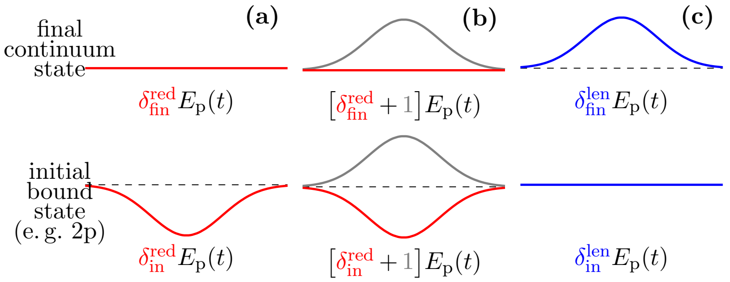


Figure S1: Sketch, analogous to Fig. 1 in the text, showing the relation between the dynamic Stark shift of the initial and final states in either reduced velocity, velocity or length gauge for a state with vanishing Stark shift (e. g. for the 2p-state of hydrogen at $\omega = 12\,\text{eV}$, where $\delta^{\text{red}}_{\text{in}} \approx -1$, $\delta^{\text{red}}_{\text{fin}} \approx 0$, $\delta^{\text{len}}_{\text{in}} \approx 0$ and $\delta^{\text{len}}_{\text{fin}} \approx +1$).

## 3 Time-dependent Schrödinger equation

In this section we will give details of the numerical calculations presented in the text.

### 3.1 Numerical propagation and spectra

The lowest $n$ field-free states of each angular momentum $\ell = 0 \ldots \ell_{\text{max}}$ are calculated numerically by means of the Numerov method in a finite box $r = 0 \ldots r_{\text{max}}$ of grid spacing $\delta r = 0.01\,\text{a}_0$. The size of the box $r_{\text{max}}$ is chosen such that the continuum wave-packet does not reach the box boundary within the propagation time ($r_{\text{max}} \approx 2000 \ldots 4000\,\text{a}_0$). The energy of the highest state for each angular momentum can be estimated as $E_{\text{max}} \approx n^2\pi^2/2r_{\text{max}}{}^2$ (e. g. for $n = 3000$ and $r_{\text{max}} = 3000\,\text{a}_0$ it is $E_{\text{max}} \approx 134\,\text{eV}$).

The dipole coupling matrix between states $j$ and $j'$, where $|\ell_j - \ell_{j'}| = 1$, with radial functions $\varphi_j$ and $\varphi_{j'}$ is calculated as $p_{jj'} = \mathrm{i}[E_j - E_{j'}]\frac{\ell}{\sqrt{4\ell^2-1}}\langle\varphi_j|r|\varphi_{j'}\rangle$ with $\ell = \max(\ell_j, \ell_{j'})$. The time-dependent

Schrödinger equation can be written in terms of these couplings as

$$\mathrm{i}\dot{a}_j(t) = \sum_{j'} \left[E_j \delta_{jj'} + \mathcal{A}(t)\, p_{jj'}\right] a_{j'}(t), \tag{S12}$$

whereby the numerical propagation is facilitated by the fact that the matrix $p_{jj'}$ has a block structure.

The electron energy spectrum for a certain channel, i.e. a certain angular momentum, is obtained using the sum

$$P_\ell(E) = \frac{1}{\sqrt{\pi}\,\sigma_E} \sum_{j(\in\ell)} \left|a_j(t_{\mathrm{fin}})\right|^2 \mathrm{e}^{-[E-E_j]^2/\sigma_E{}^2} \tag{S13}$$

where typically $t_{\mathrm{fin}} = 3T$ and $\sigma_E = 0.025\,\mathrm{eV}$. The sum over $j$ is restricted to all states with the same angular momentum $\ell$.

### 3.2 Velocity vs. length gauge

For comparison one can perform calculations in the length gauge by means of a similar method. The equations to be solved are

$$\mathrm{i}\dot{a}_j(t) = \sum_{j'} \left[E_j \delta_{jj'} - \tfrac{\mathrm{d}}{\mathrm{d}t}\mathcal{A}(t)\, d_{jj'}\right] a_{j'}(t), \tag{S14}$$

where $d_{jj'} = \frac{\ell}{\sqrt{4\ell^2-1}} \langle \varphi_j | r | \varphi_{j'} \rangle$ with $\ell = \max(\ell_j, \ell_{j'})$.

Figure S2 shows results of simulations with the largest partial wave $\ell_{\max}$ included going well above what has been used before [1, 4–6]. It can be seen that even for $\ell_{\max} = 32$ the spectrum is not converged in the length gauge, while it only requires $\ell_{\max} = 1$ for convergence in the velocity gauge. One also recognizes the false dynamic interference appearing for low $\ell_{\max}$ in the length gauge which is an artifact of the non-converged results. These non-converged results effectively mimic the behaviour of a system in which the continuum states undergo no stark shift; a direct consequence of the lack of enough partial waves required for accommodating the dependence of the stark shift of the continuum states on the ponderomotive energy in the length gauge. Obviously the effective Stark shift calculated using these results is wrong or more specifically it is exaggerated.

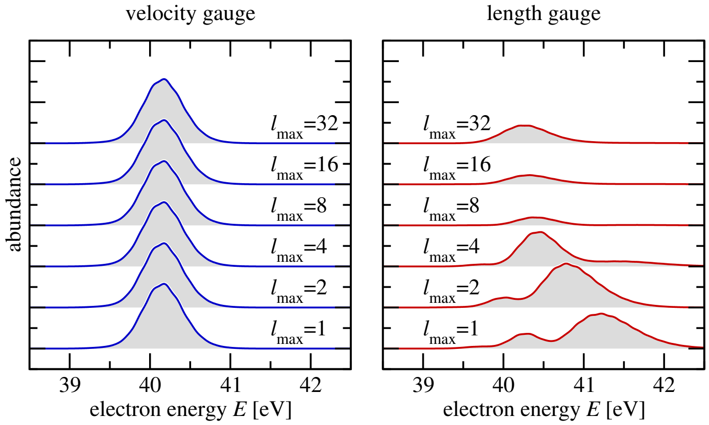


Figure S2: Comparison of photoelectron spectra obtained in the velocity and the length gauges for $T = 3\,\mathrm{fs}$, $I = 5{\times}10^{16}\mathrm{W/cm^2}$ and $\omega = 53.6\,\mathrm{eV}$.

## References


[1] P. V. Demekhin and L. S. Cederbaum, *ac Stark effect in the electronic continuum and its impact on the photoionization of atoms by coherent intense short high-frequency laser pulses*. Phys. Rev. A 88, 043414 (2013).

[2] M.H. Mittleman, *Introduction to the theory of laser-atom interactions* (Plenum Press, New York and London, 1993).

[3] R. Jackiw, *Quantum-mechanical sum rules*. Phys. Rev. 157, 1220 (1967).

[4] P. V. Demekhin and L. S. Cederbaum, *Dynamic interference of photoelectrons produced by high-frequency laser pulses*. Phys. Rev. Lett. 108, 253001 (2012).

[5] P. V. Demekhin, D. Hochstuhl, and L. S. Cederbaum, *Photoionization of hydrogen atoms by coherent intense high-frequency short laser pulses: Direct propagation of electron wave packets on large spatial grids*. Phys. Rev. A 88, 023422 (2013).

[6] C. Yu, N. Fu, G. Zhang, and J. Yao, *Dynamic Stark effect on XUV-laser-generated photoelectron spectra: Numerical experiment on atomic hydrogen*. Phys. Rev. A 87, 043405 (2013).
